# Supplementary material for: Semantically Consistent Video Inpainting with Conditional Diffusion Models
Source: arXiv:2405.00251 source file (2024-10-08)
Supplement: Supplementary file 1 [file algorithms.tex]

\section{Algorithms}
\hlr{UPDATE TO DEAL WITH Z}

\begin{algorithm}[h]
\caption{Training}
\label{alg:train}
\begin{algorithmic}[1]
\Repeat
\State $(\bV, \bM) \sim q(\bV, \bM)$\Comment{Sample video and mask}
\State $(\mathcal{X}, \mathcal{Y}) \sim u(\mathcal{X}, \mathcal{Y})$\Comment{Sample training task}
\State $t \sim \mathcal{U}(\{1 \ldots T\})$
\State $\boldsymbol{\epsilon} \sim \mathcal{N}(\mathbf{0}, \mathbf{I})$
\State $(\bV', \bM') \gets (\bV[\fX \cup \fY], \bM[\fX \cup \fY])$\Comment{Extract selected frames}
\State $\bV_t' \gets \sqrt{\bar{\alpha}_t}\bV' + \sqrt{1-\bar{\alpha}_t}(\mathbbm{1}-\bM')\odot\boldsymbol{\epsilon}$\Comment{Noise latent pixels}
\State Take gradient descent step on \newline
\hspace*{3em}$\nabla_\theta \|(1-\bM')\odot(\boldsymbol{\epsilon} - \boldsymbol{\epsilon}_\theta(\bV_t', \bM', \mathcal{X}, \mathcal{Y}, t))\|^2$\Comment{Masked loss}
\Until converged
\end{algorithmic}
\end{algorithm}

\begin{algorithm}[h]
\caption{Inpaint video $\bV$ given mask $\bM$ and sampling scheme $\left[(\mathcal{X}_s, \mathcal{Y}_s)\right]^S_{s=1}$}
\label{alg:alg}
\begin{algorithmic}[1]
\For{$s \gets 1, \ldots, S$}
\State $\bV_s' \gets \bV [\fX_s \cup \fY_s]$\Comment{Extract selected video frames}
\State $\bM_s' \gets \bM [\fX_s \cup \fY_s]$\Comment{Extract selected mask frames}
\State $\hat{\bV}_s \sim \texttt{DDPM}(\cdot;\bV_s', \bM_s', \mathcal{X}, \mathcal{Y},\theta)$\Comment{Sample}
\State $\bV [\fX_s \cup \fY_s] \gets \hat{\bV}_s$\Comment{Insert completed frames}
\State $\bM [\fX_s] \gets \mathbbm{1}$\Comment{Update masks for inpainted frames}
\EndFor
\State \Return $\bV$
\end{algorithmic}
\end{algorithm}
